# Supplementary material for: Data-driven discovery of dynamics from time-resolved coherent scattering
Source: arXiv:2311.14196 source file (2024-09-20)
Supplement: Supplementary file 1 [file supp.tex]

% Supplementary Material
\clearpage
\clearpage

\setcounter{section}{0}
\setcounter{equation}{0}
\setcounter{figure}{0}
\setcounter{table}{0}
\setcounter{page}{1}
\makeatletter

\title{\vspace{-1.5cm}\Large Supplemental Material for "Data-driven discovery of dynamics from time-resolved coherent scattering"}
\date{}
\maketitle
